# Supplementary material for: Formal Explanations for Neuro-Symbolic AI
Source: arXiv:2410.14219 source file (2024-10-18)
Supplement: Supplementary file 1 [file appendix.tex]

\appendix

% \section{Appendix / Supplemental Material}

%%%%%%%%%%%%%%%%%%%%%%%%%%%%%%%%%%%%%%%%%%%%%%%%%%%%%%%%%%%%

\newpage
